# Supplementary material for: Raman evidence for nonadiabatic effects in optical phonon self-energies of transition metals
Source: arXiv:1611.10006 source file (2016-11-30)
Supplement: Supplementary file 1 [file supp_info.pdf]

# Raman evidence for nonadiabatic effects in optical phonon self-energies of transition metals

*Yu. S. Ponosov*[1,2] *and S. V. Streltsov*[1, 2]

[1]M. N. Mikheev Institute of Metal Physics UB RAS, 620990 Ekaterinburg, Russia
[2]Ural Federal University, 620002 Ekaterinburg, Russia

**Supplementary Information**

1. **Phonon density of states in Os**
2. **Cross-section of yttrium Fermi surface**
3. **Raman spectra of investigated metals**

## 1. Phonon density of states in Os

There are no experimental data on the phonon spectra of Os. Therefore, we used our second order Raman spectra of Os plotted in ω/2 scale for our calculations (Fig.S1.

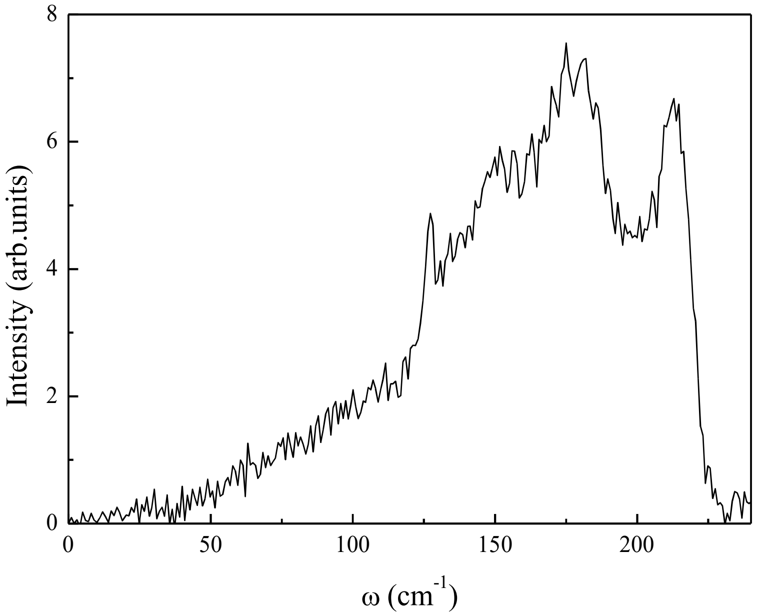


Fig.S1. Phonon density of states in Os obtained from two-phonon spectrum.

## 2. Cross-section of yttrium Fermi surface

Low-temperature difference of the phonon energies for different q-directions is due to the difference of average bare electron velocities **ʋ** on the Fermi surface for probed q-directions. In its turn, **ʋ** for a probed q- direction is determined by both an electron velocity and the Fermi surface shape, which sets the value of the average velocity for this q- direction. So, yttrium has a "webbing" Fermi surface which looks as open (along axis) corrugated cylinder with "webbing" near AHL basal plane (see Fig.S2 ). Although the maximum velocity for the third sheet of the Fermi surface was found for q-direction in the basal plane ($\upsilon_x$ and $\upsilon_y$), it occurs only in a small part of a cylindrical surface. On the flat surface of "webbing" the velocity for q- direction along the crystal axis ($\upsilon_z$) is slightly smaller, but practically invariable. Because the area of "webbing" is several times larger

than the area of this small part of cylindrical surface, the average velocity for q - direction along the axis exceeds the velocities for q-directions in the basal plane. This follows from our calculation.

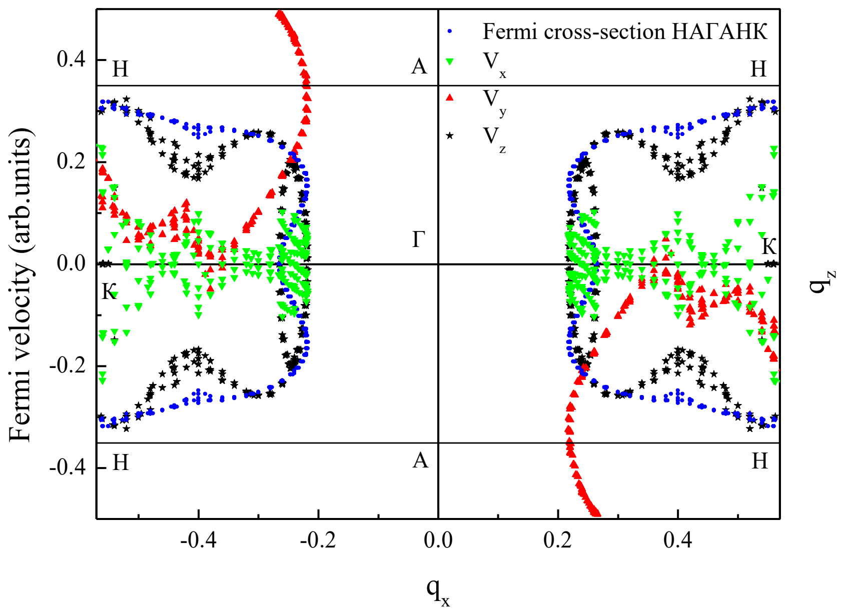


Fig.S2 Cross-section of third band sheet of the Fermi surface in yttrium (ΓKHA plane). Left axis shows values of different components of Fermi velocity at this sheet (triangles –in basal plane, star – along crystal axis).

### 3. Raman spectra of investigated metals

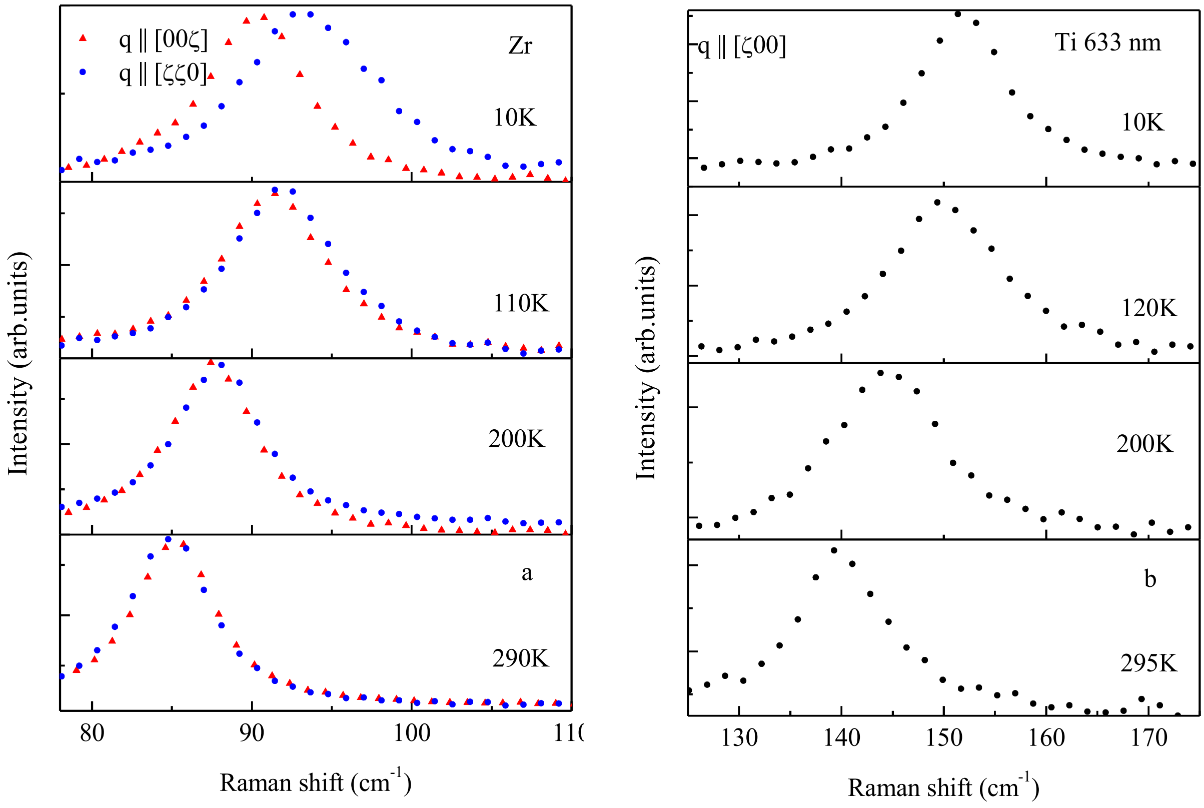


Fig. S3. Measured Raman spectra of Zr (a) and Ti (b) at different temperatures.

We show measured spectra of investigated metals Zr, Ti, Ru and Os in Figs. S3-S5.

For titanium (Fig.S3,b) Raman spectra are shown only for one probed q-direction because the phonon line shapes for all q-directions are hard to distinguish.

In case of Ru (Fig.S4) the measured spectra are plotted together with the calculated ones. The last show significant broadening compared with the experimental spectra since both adiabatic and nonadiabatic regions of the phonon spectrum give large contributions to phonon line shape. Nevertheless, dominating features in calculated spectral functions are close to the energies of experimental peaks.

For osmium (Figs. S5) measured phonon profiles are shown for two excitation wavelengths 514 and 647 nm after subtracting of the electronic background that was presented in Fig.7 of the article. An obvious change of the difference in the frequencies of longitudinal and transverse phonons with q- vector in the basal plane is observed when the excitation wavelength varies.

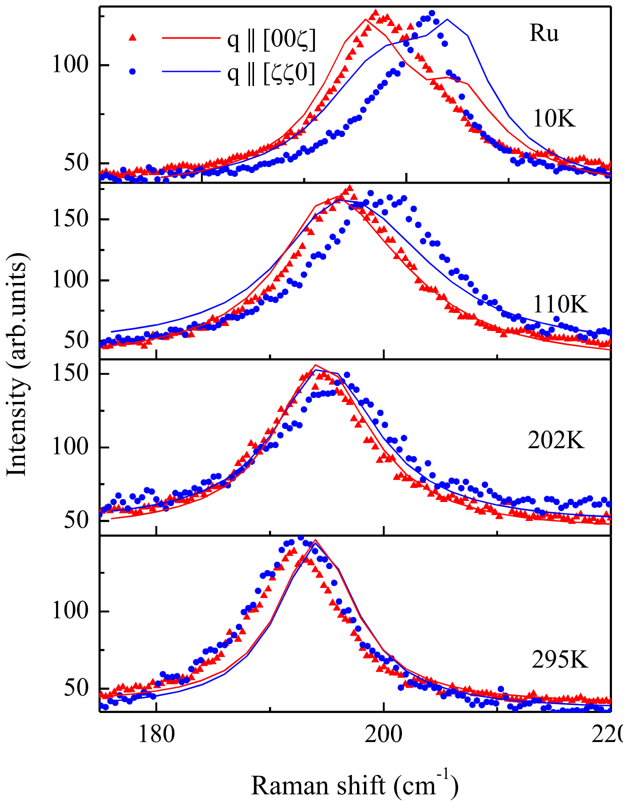


Fig. S4. Measured and calculated spectra of Ru for two q-directions at different temperatures.

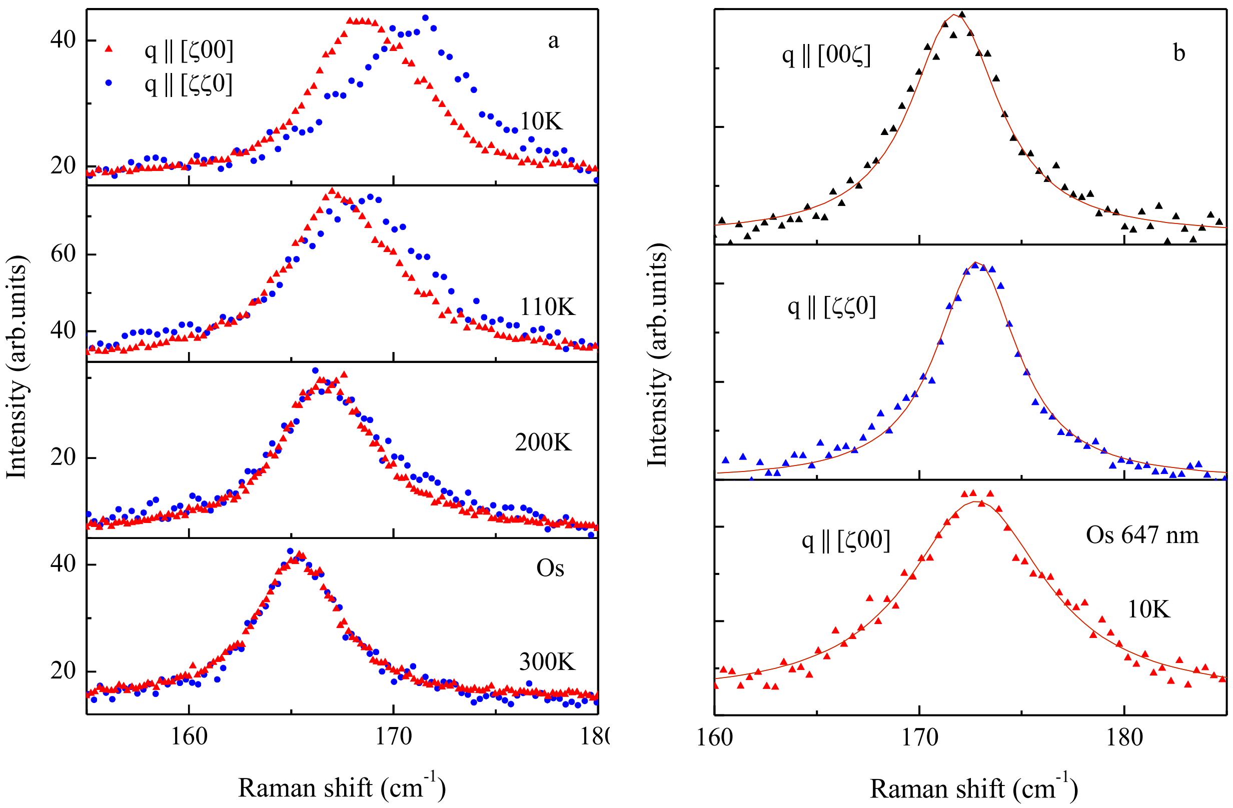


Fig. S5. Phonon profiles in Os at excitation 514 nm (a) and 647 nm (b) for different q-directions.
